# Supplementary material for: Sensing Resource Allocation Against Data-Poisoning Attacks in Traffic Routing
Source: arXiv:2404.02876 source file (2024-09-11)
Supplement: Supplementary file 1 [file appendix.tex]

\appendix

\subsection{Best response flow (complete information)}
\label{app:coefficients}

We will briefly elaborate upon our computation in (\ref{eq:best_response_flow_polynomial}, and provide the coefficients $\zeta^i_{j,k}$ for the best response flow for a given attack $t=i$. 
Recall we had:

\begin{align}
\label{eq:app.best_response.a}
    \nonumber \mathbb{E} &\left[ \sum_{j=1}^{n_l} \phi_j(y_j ; f_j) \; \bigg| \; t=i \right] \\
    % \nonumber =& \sum_{j=1}^{n_l}\mathbb{E} \left[ \phi_j (y_j ; f_j) \; \bigg| \; t=i \right] \\
    =& \sum_{j=1}^{n_l} b_j y_j + \frac{y_j}{c_j^4} \; \mathbb{E} \left[ \left( a^i_j - (\hat{f}_j + y_j) \right)^4 \right]
\end{align}
Since $a^i_j - (\hat{f}_j + y_j) \sim \mathcal{N}(\mu_j^i - (\hat{f}_j + y_j), \sigma_j^i),$ we may compute this moment as
% \begin{equation}
%          \mathbb{E} \left( a^i_j - (\hat{f}_j + y_j) \right)^4
%          =  \sum_{k=0}^2 {4 \choose 2k } (y_j - \tilde{\mu}_j^i)^{2k} (\sigma_j^i)^{4-2k} 
% \end{equation}
\begin{align}
         \nonumber \mathbb{E}& \left( a^i_j - (\hat{f}_j + y_j) \right)^4 \\
         &= 3(\sigma_j^i)^2 + 6 (\sigma_j^i)(y_j - \tilde{\mu}_j^i)^2 + (y_j - \tilde{\mu}_j^i)^4
         % =  \sum_{k=0}^2 {4 \choose 2k } (y_j - \tilde{\mu}_j^i)^{2k} (\sigma_j^i)^{4-2k} 
\end{align}
where we let $\tilde{\mu}_j^i = \mu_j^i - \hat{f}_j$.
By plugging into Eq.~(\ref{eq:app.best_response.a}), we may gather the coefficients for the  best response flow for attack $i$, as in Eq.~(\ref{eq:best_response_flow_polynomial}):
\begin{subequations}
\begin{align}
    \zeta^i_{j,1} &= {\left(b_j + \frac{(\tilde{\mu}_j^i)^{4}}{c_j^{4}} + \frac{6 \, (\tilde{\mu}_j^i)^{2} (\sigma_j^i)^{2}}{c_j^{4}} + \frac{3(\sigma_j^i)^{4}}{c_j^{4}}\right)} \\
    \zeta^i_{j,2} &= - 4 \, {\left(\frac{(\tilde{\mu}_j^i)^{3}}{c_j^{4}} + \frac{3 \, (\tilde{\mu}_j^i) (\sigma_j^i)^{2}}{c_j^{4}}\right)} \\
    \zeta^i_{j,3} &= 6 \, {\left(\frac{(\tilde{\mu}_j^i)^{2}}{c_j^{4}} + \frac{(\sigma_j^i)^{2}}{c_j^{4}}\right)}\\
    \zeta^i_{j,4} &= - \frac{4 \, (\tilde{\mu}_j^i)}{c_j^{4}}\\
    \zeta^i_{j,5} &= \frac{1}{c_j^{4}}
\end{align}
\end{subequations}

\subsection{Bayesian optimal routing (incomplete information)}
In this appendix, we derive the coefficients $\eta_{j,k}$ and $\kappa_{j,k}$ in (\ref{opt: bayesian routing expanded}) by computing the expected cost from (\ref{opt: bayesian routing}). We begin by considering the distribution with respect to which we take the expectation in (\ref{opt: bayesian routing}).
Since we have directly observed $f_i$ for $i \in o$, we make take those values as given and only worry about taking the expectation for $f_i$ with $i \in \bar{o}$, i.e. we factor our posterior distribution over $f$ into the observed and unobserved components:\;
\begin{align}
    \label{eq:app.full posterior f}
    p \left(f' \; \bigg| \; \hat{f}, a_{o} \right) = \delta_{f
    _{o(x)}}(f'_{o}) \; p \left(f_{\bar{o}}' \; \bigg| \; \hat{f}, a_{o} \right)
\end{align}
where we're using the dummy vector $f'$ to avoid the potentially confusing abuse of notation $\delta_{f_{o(x)}}(f_{o(x)})$.

Then the objective in Eq.~(\textcolor{red}{ZZZ}) is given by
\begin{align}
    &\nonumber \underset{p' \left(f | \hat{f}, a_{o} \right)}{\mathbb{E}} \left( \sum_{j=1}^{n_l} \phi_j(y_j ; f'_j) \right) \\
    \nonumber &= \sum_{j \in o} \phi_j(y_j; f_j) + \underset{p' \left(f_{\bar{o}} | \hat{f}, a_{o} \right)}{\mathbb{E}} \sum_{j \in \bar{o}} \phi(y_j ; \hat{f}_j - a_j)
\end{align}

\todo[inline]{Old version of the text}

In this appendix, we derive the coefficients $\eta_{j,k}$ and $\kappa_{j,k}$ in (\ref{opt: bayesian routing expanded}) by computing the expected cost from (\ref{opt: bayesian routing}).

We begin by considering the distribution with respect to which we take the expectation in (\ref{opt: bayesian routing}).
Since we have directly observed $f_i$ for $i \in o$, we make take those values as given and only worry about taking the expectation for $f_i$ with $i \in \bar{o}$, i.e. we factor our posterior distribution over $f$ into the observed and unobserved components:\;
\begin{align}
    \label{eq:app.full posterior f}
    p \left(f' \; \bigg| \; \hat{f}, a_{o} \right) = \delta_{f
    _{o(x)}}(f'_{o}) \; p \left(f_{\bar{o}}' \; \bigg| \; \hat{f}, a_{o} \right)
\end{align}
Since it is always given, we omit $\hat{f}$ from our distributional notation for the rest of this section.
Moreover, it will be easier to instead consider

Let's begin with the unobserved component $p(f_{\bar{o}} | a_{o})$.
This distribution is more easily represented over $a_{\bar{o}}$ in place of $f_{\bar{o}}$.
\begin{equation}
    \label{eq:app.p abaro given ao}
    p( a_{\bar{o}} \; | \; a_{o} )
    = \sum_{t} p( a_{\bar{o}} \; | \: t, a_{o}) \; P(t \; | \; a_{o})
\end{equation}
where $p( a_{\bar{o}} \; | \: t, a_{o})$ is the conditional Gaussian density on $a_{\bar{o}}$ for a given attack $t$, and $P(t \; | \; a_{o})$ is the posterior pmf over the attack types.
Using Bayes' rule, we expand the posterior:
\begin{align}
    P(t | a_{o}) = \frac{p(a_{o} | t)\; P(t)}{p(a_{o})}
\end{align}
% which is related to the distribution in ()
If we assume a uniform prior $P(t) = 1/n_a$, then we have that
\begin{equation}
    P(t | a_{o}) \propto p(a_{o} | t)
\end{equation}
% Note that this tells us that the frequentist and Bayesian perspectives align under the uniform prior, since () implies that the MLE and MAP estimate of $t$ are identical.
We may then use the attack type likelihood $p(a_{o} | t)$ in place of the posterior for integrating the optimization problem (\ref{opt: bayesian routing}), i.e. we can integrate over the unnormalized density
\begin{equation}
q(a_{\bar o} \; | \; a_{o}) = \sum_{t} p( a_{\bar{o}} \; | \: t, a_{o}) \; p(a_{o} | t)
\end{equation}
which is related to $p( a_{\bar{o}} | a_{o} )$ from (\ref{eq:app.p abaro given ao}) via the normalization constant:
\begin{align}
    q(a_{\bar{o}} | a_{o}) &= Z(a_{o}) p(a_{\bar{o}} | a_{o}) \\
    Z(a_{o}) &\triangleq \sum_t p(a_o|t)
\end{align}
% In fact, we will need to multiply the full distribution in (\ref{eq:app.full posterior f}) by $Z(a_{o})$.

The likelihood of the attack type is given by the Gaussian density
\begin{equation}
    % g(a_{\bar{o}}) \triangleq
    p(a_{o} | t) = \mathcal{N}_{a_{o}}(O \mu^t, \Sigma^t_{oo})
\end{equation}
where $\Sigma^t_{oo} = O \Sigma^t O^\top$.
The conditional distribution $p( a_{\bar{o}} | t, a_{o})$ takes the form
\begin{subequations}
\label{eq:conditional posterior per type}
\begin{equation}
    p( a_{\bar{o}} \; | \; t, a_{o} ) = \mathcal{N}_{a_{\bar{o}}}(\omega^t, \Omega^t)
\end{equation} \begin{align}
% \mu^t_{o | \bar o}
\omega^t
% = \omega^t(o | \bar o)
&= \bar{O} \mu^t + \Sigma^t_{\bar{o}o} (\Sigma^t_{oo})^{-1}(a_{o} - O\mu^t)\\
 % \Sigma^t_{o | \bar o}
 \Omega^t
 &= \Sigma_{\bar{o} \bar{o}} - \Sigma^t_{\bar{o} o} \Sigma^t_{oo} (\Sigma^t_{\bar{o} o})^{-1}
 % \intertext{where}
 % \Sigma^t_{\bar{o} \bar{o}} &= \bar{O} \Sigma^t \bar{O}^\top \\
 % \Sigma^t_{\bar{o} o} &= \bar{O} \Sigma^t O^\top \\
 %  \Sigma^t_{o o} &= O \Sigma^t O^\top
\end{align}
\end{subequations}
where $\Sigma^t_{\bar{o} \bar{o}} = \bar{O} \Sigma^t \bar{O}^\top$ and $\Sigma^t_{\bar{o} o} = \bar{O} \Sigma^t O^\top$.
\label{appendix:bayesian routing}

Now we have all the component pieces we need to compute the problem in \ref{opt: bayesian routing}.
We are finding the solution for the equivalent problem
\begin{equation}
\label{opt: bayesian routing unnormalized}
\begin{array}{ll}
\underset{y, z}{\mbox{minimize}} &  
\int \left( \sum_{j=1}^{n_l} \phi_j(y_j ; \hat{f}_j - a'_j) \right) q(a' \;;\; a_o) da \\
% \sum_{j=1}^{n_l} \left(b_j+ \left(\frac{f_j+y_j}{c_j}\right)^4\right)y_j\\
\mbox{subject to} & Hz=d, \, Fz=y, z\geq 0_{n_r}.
\end{array}
\end{equation}
where our unnormalized distribution is given as $q(a' \,;\, a_o) = \delta_{a_o}(a'_o) q(a'_{\bar{o}} ; a'_{o})$.
We break this objective function up into the observed ($a_o$-dependent) and unobserved ($a_{\bar{o}})$-dependent) components:
\begin{align}
\label{eq: appendix breakout bayesian routing}
\nonumber    & \int \left( \sum_{j=1}^{n_l} \phi_j(y_j ; \hat{f}_j - a'_j) \right) q(a' \;;\; a_o) da \\
\nonumber    &= Z(a_o) \sum_{j \in o} \phi_j(y_j; \hat{f}_j - a_j)  \\
    &+ \sum_{t} p(a_o | t) \sum_{j \in \bar{o}} \int \phi_j(y_j; \hat{f}_j - a_j) p( a_j \; | \; t, a_{o} ) d a_j
\end{align}
where $p( a_j \, | \, t, a_{o} )$ are just the univariate component distributions of $ p( a_{\bar{o}} \; | \; t, a_{o} )$ from (\ref{eq:conditional posterior per type}a-c).

Let's compute the second term. Similar to (\ref{eq:app.best_response.a}), we have

\begin{align}
    \nonumber & \int  \phi_j(y_j; \hat{f}_j - a_j) \; p( a_j \; | \; t, a_{o} ) d a_j \\
    =&  \quad b_j y_j + \frac{y_j}{c_j^4} \; \int 
    \left( a^i_j - (\hat{f}_j + y_j) \right)^4 p( a_j \; | \; t, a_{o} ) \, da_j
\end{align}

Since $a^i_j - (\hat{f}_j + y_j) \sim \mathcal{N}(\omega^t_j - (\hat{f}_j + y_j), \Omega^t_{jj})$, we use the same formula as before, letting $\tilde{\omega}^t_j = \omega^t_j$. Then we have that
\begin{subequations}
\begin{equation}
    \int  \phi_j(y_j; \hat{f}_j - a_j) \; p( a_j \; | \; t, a_{o} ) d a_j
    = \sum_k \tilde{\kappa}_{j,k,t} \; y_j^k
\end{equation}
where
\begin{align}
    \tilde{\kappa}_{j,1,t} &= {\left(b_j + \frac{(\tilde{\omega}_j^t)^{4}}{c_j^{4}} + \frac{6 \, (\tilde{\omega}_j^t)^{2} (\Omega_{jj}^t)^{2}}{c_j^{4}} + \frac{3(\Omega_{jj}^t)^{4}}{c_j^{4}}\right)} \\
    \tilde \kappa_{j,2,t} &= - 4 \, {\left(\frac{(\tilde{\omega}_j^t)^{3}}{c_j^{4}} + \frac{3 \, (\tilde{\omega}_j^t) (\Omega_{jj}^t)^{2}}{c_j^{4}}\right)} \\
    \tilde \kappa_{j,3,t} &= 6 \, {\left(\frac{(\tilde{\omega}_j^t)^{2}}{c_j^{4}} + \frac{(\Omega_{jj}^t)^{2}}{c_j^{4}}\right)}\\
    \tilde \kappa_{j,4,} &= - \frac{4 \, (\tilde{\omega}_j^t)}{c_j^{4}}\\
    \tilde \kappa_{j,5,t} &= \frac{1}{c_j^{4}}
\end{align}
\end{subequations}
This gives us the second term on the RHS of (\ref{eq: appendix breakout bayesian routing}), and in turn the coefficients $\kappa_{j,k}$ in (\ref{opt: bayesian routing expanded}):

\begin{subequations}
    \label{eq: appendix bayesian routing unobserved terms}
\begin{gather}
    \nonumber \sum_{t} p(a_o | t) \sum_{j \in \bar{o}} \int \phi_j(y_j; \hat{f}_j - a_j) p( a_j \; | \; t, a_{o} ) d a_j \\ = \sum_k \kappa_{j,k} y_j^k
\end{gather}
where
\begin{align}
    \kappa_{j,k} &= \sum_t \mathcal{N}_{a_o}(O \mu^t, \Sigma^t_{oo}) \tilde{\kappa}_{j,k,t}
\end{align}
\end{subequations}
Note that this Gaussian density $\mathcal{N}_{a_o}(O \mu^t, \Sigma^t_{oo})$ takes the form
\begin{subequations}
\begin{align}
    \mathcal{N}_{a_o}(O \mu^t, \Sigma^t_{oo}) &= \frac{1}{(2 \pi)^{|o|/2} |\Sigma^t_{oo}|^{1/2}} \exp \left( - \frac{1}{2} \left\| a_o - O \mu^t \right\|^2_{\Sigma^t_{oo}} \right) \\
    \left\| a_o - O \mu^t \right\|^2_{\Sigma^t_{oo}} &= (a_o - O\mu^t)^\top (\Sigma^t_{oo})^{-1} (a_o - O\mu^t)
\end{align}
\end{subequations}

The first term on the RHS of (\ref{eq: appendix breakout bayesian routing}) just expands the costs defined by (\ref{eq: cost kernel}) for the directly observed edges, with ambient traffic $f_j = \hat{f}_j - a_j$.
For each edge, this is:
\begin{equation}
    \phi_j(y_j ; f_j) = b_j y_j + \frac{y_j}{c_j^4} \sum_{k=0}^4 {4 \choose k} f_j^{4-k} y_j^k
\end{equation}
and thus we have our coefficients:
\begin{subequations}
\label{eq: appendix bayesian routing observed terms}
\begin{equation}
    Z(a_o) \sum_{j \in o} \phi_j(y_j; \hat{f}_j - a_j) = \sum_k \eta_{j,k} y_j^k
\end{equation}
where
\begin{align}
    \eta_{j,1} &= Z(a_o) \left( b_j + \left( \frac{f_j}{c_j} \right)^4 \right) \\
    \eta_{j,k} &= Z(a_o) {4 \choose k-1} \frac{f_j^{5-k}}{c_j^4}
    \quad \text{ for } k\geq 2 \\[6pt]
    Z(a_o) &= \sum_t \mathcal{N}_{a_o}(O \mu^t, \Sigma^t_{oo})
    % \eta_{j,2} &= 4\frac{f_j^3}{c_j^4}\\
    % \eta_{j,1} &= 6\frac{f_j^2}{c_j^4}\\
    % \eta_{j,1} &= 4\frac{f_j}{c_j^4}\\
    % \eta_{j,1} &= \frac{1}{c_j^4}\\
\end{align}
\end{subequations}

Thus, putting together (\ref{eq: appendix bayesian routing unobserved terms}) and (\ref{eq: appendix bayesian routing observed terms}) to get the objective function (\ref{eq: appendix breakout bayesian routing}), we have the problem formulation (\ref{opt: bayesian routing expanded}), and the exact forms of our coefficients $\eta_{j,k}$ and $\kappa_{j,k}$.
